# Supplementary material for: Synchronization of coupled Kuramoto oscillators competing for resources
Source: arXiv:2206.02851 ancillary file (2022-06-06)
Supplement: Supplementary file 1 [file ResourceCompetitionSupplement.pdf]

# Supplemental Information

## 1 Biased Random Walk with Negative Bias

Consider a biased random walk dynamics

$$\dot{B}_i = p \sum_j C_{ij} (B_j b_i - B_i b_j) \,, \tag{1}$$

where $b_i$ are the biases.

Suppose, for the sake of this discussion, that the biases are fixed. Then the equilibrium distribution of resources will simply be

$$B_i = k b_i \,, \tag{2}$$

since this will immediately make $\dot{B}_i$ equal to zero.

Now due to the fixed total supply of $B_i$, we also must apply the condition

$$\sum_i B_i = B_{\text{tot}} \,. \tag{3}$$

If we apply this condition here, we can solve for $k$, and we find

$$k = \frac{B_{\text{tot}}}{\sum_i b_i} \,. \tag{4}$$

Thus, we find that it will be far simpler if we disallow the possibility of negative biases, since such negative biases introduce the possibility that the denominator could be zero. For this reason, in our analysis, we introduce the $\tilde{\omega}$ term to drag all net frequencies above zero.

## 2 Frequencies remain greater than 0

One may naturally wonder if the introduction of the $\tilde{\omega}$ term is really sufficient to accomplish the task of keeping $\dot{\phi}_i > 0$ at all times. Technically, all we control is the initial state of the system, so we would like to show that, as long as $\dot{\phi}_i > 0$ in the initial state, then it will remain that way in all future states.

To see this, first consider the dynamics in the case of no phase coupling.

$$\dot{\phi}_i = \tilde{\omega} + \tilde{\sigma}\omega_i' + \tilde{\mu}R_i' \tag{5}$$

$$\dot{R}_i' = B_i' - R_i' + \tilde{\beta}\dot{\phi}_i \tag{6}$$

$$\dot{B}_i' = p\sum_j C_{ij}(B_j'\dot{\phi}_i - B_i'\dot{\phi}_j)\,. \tag{7}$$

Now, suppose that the initial state of $R_i'$ is such that $\dot{\phi}_i$ is initially zero, and also naturally that $B_i' > 0$ for all $i$, which stems from the lack of negative biases.

Now, if $\tilde{\beta} > 0$ and, by assumption, $\dot{\phi}_i > 0$, then $\dot{R}_i'$ will only have one negatively-contrubuting term, which is $R_i'$, and so as $R_i'$ approaches zero, $\dot{R}_i'$ will always eventually be positive, so $R_i' > 0$ at all times, which means as long as $\tilde{\mu} > 0$ (which it always is in our simulations), $\dot{\phi}_i$ will always be greater than zero. The only exception would be if $\tilde{\sigma} > \tilde{\omega}$, but as explained in the main paper, we intentionally choose $\tilde{\omega} > \tilde{\sigma}$ to avoid such cases.

Now what if $\tilde{\beta} < 0$? In that case, we can find that $\dot{R}_i' < 0$ even when $R_i' = 0$ as a result of the extra negatively-contributing term. However, if we ever run into a situation where $\dot{\phi}_i$ is approaching zero, the extra negatively-contributing term will also approach zero, and so we will find that $\dot{R}_i'$ will be positive, so that $R_i'$ will increase, and therefore $\dot{\phi}_i$ will increase, once again avoiding a negative value. If we want to be a bit more precise, we may plug Equation 5 into Equation 6 to find

$$\dot{R}_i' = B_i' + \tilde{\beta}\tilde{\omega} + \tilde{\beta}\tilde{\sigma}\omega_i' + (1 + \tilde{\beta}\tilde{\mu})R_i'\,. \tag{8}$$

Here we see that the first three terms are necessarily positive in the aggregate, so $R_i'$ will always be greater than zero, which entails that $\dot{\phi}_i$ will always be greater than zero. So we find that, in the absence of coupling, as long as $\dot{\phi}_i > 0$ initially, it will remain that way at all future times given the constraints we have placed on parameter values.

Finally, we consider the case in which coupling is present. In this case, we actually do occasionally find negative values for $\dot{\phi}_i$. However, these do not spell any great danger for divergence in the bias terms because the coupling is equal and opposite. Thus, whenever one oscillator acts on another, their velocities are increased and decreased in equal quantity, so that the sum of the bias terms $\dot{\phi}_i$, which is the quantity responsible for any divergence, will keep precisely the same value with or without the coupling. Hence, we find that the divergence is avoided, whether or not there is coupling, so long as all the natural frequencies are initially positive.

# 3 Analysis Section Derivations

## 3.1 Doubly-Synchronized

We begin with the doubly-synchronized state. In this state, we take the limit as both $K_{12}$ and $K_{34}$ tend toward infinity. In this limit, any two oscillators

which are connected in the phase-coupling layer will be perfectly in-sync with one another. Thus, all of the {G1,G2} oscillators will move at one frequency $\Omega_{12}$, and all of the {G3,G4} oscillators will move at another frequency $\Omega_{34}$. First, we will prove that these must actually be the same frequency.

Beginning with the dynamical equations under the assumption that oscillators move at either $\Omega_{12}$ or $\Omega_{34}$ depending on group membership, we then have

$$\dot{\phi}_i = \Omega_{12/34} \tag{9}$$

$$\dot{R}'_i = B'_i - R'_i + \tilde{\beta}\dot{\phi}_i \tag{10}$$

$$\dot{B}'_i = p \sum_j C_{ij} (B'_j \dot{\phi}_i - B'_i \dot{\phi}_j)\,. \tag{11}$$

Naturally we can replace the $\dot{\phi}_i$ terms by $\Omega_{12/34}$. If we then solve for the equilibrium $B'_i$, we find

$$B'_i = \frac{\dot{\phi}_i}{\sum_j \dot{\phi}_j} = \frac{1}{N} \frac{\Omega_{12/34}}{\Omega_{12} + \Omega_{34}}\,. \tag{12}$$

We can then use this to solve for the equilibrium $R'_i$, and we find

$$R'_i = \frac{1}{N} \frac{\Omega_{12/34}}{\Omega_{12} + \Omega_{34}} + \tilde{\beta}\Omega_{12/34}\,. \tag{13}$$

Next we note that the group frequencies will necessarily just be the average natural frequency of all of the oscillators within either the {G1,G2} group or the {G3,G4} group since the coupling term is equal and opposite among pairs of oscillators. Thus, we also have the following equations

$$\Omega_{12/34} = \langle \tilde{\omega} + \tilde{\sigma}\omega'_i + \tilde{\mu} R'_i \rangle\ , \tag{14}$$

where the average is taken over either {G1,G2} or {G3,G4}, respectively.

We can simplify this equation and find

$$\Omega_{12/34} = \tilde{\omega} + \tilde{\sigma}\,\langle \omega'_i \rangle + \tilde{\mu}\,\langle R'_i \rangle\ . \tag{15}$$

Now, since the $\omega'_i$ are drawn according to a Gaussian distribution with mean 0 (at least in aggregate when considering both groups in a pair), the second term will be, in the limit of many oscillators, very nearly zero. Thus, the group frequencies are, to good approximation

$$\Omega_{12/34} = \tilde{\omega} + \tilde{\mu}\,\langle R'_i \rangle\ . \tag{16}$$

Now we can look back at Equation 13. Because of the equal frequencies of all oscillators within {G1,G2} or {G3,G4}, the internal resource levels of all oscillators within one of these pairs are equal, and equal to the level given in

Equation 13. Thus, Equations 13 and 16 give us two equations in two unknowns, $\Omega_{12}$ and $\Omega_{34}$. We can write these equations succinctly as

$$\Omega_{12/34} = \tilde{\omega} + \tilde{\mu}\left(\frac{1}{N}\frac{\Omega_{12/34}}{\Omega_{12}+\Omega_{34}} + \tilde{\beta}\Omega_{12/34}\right). \tag{17}$$

Now, because of the denominator $\Omega_{12} + \Omega_{34}$, these equations will generally result in a pair of mixed up quadratic equations in $\Omega_{12}$ and $\Omega_{34}$. That said, it is quite clear at a glance that the equations are perfectly symmetric under the interchange of (12) and (34) labels. Thus, any value which solves the equation for $\Omega_{12}$, the same value must also solve the equation for $\Omega_{34}$, since the equations are equivalent except for an interchange of labels. The only caveat is that if multiple solutions exist to this equation, then the two could in principle take on different solutions. Thus, we can rearrange Equation 17 into the following form

$$\Omega_{12/34} = \tilde{\omega}\left(1 - \tilde{\beta}\tilde{\mu} - \frac{\tilde{\mu}}{N}\frac{1}{\Omega_{12}+\Omega_{34}}\right)^{-1}. \tag{18}$$

In this form, it is perfectly clear that $\Omega_{12}$ and $\Omega_{34}$ cannot possibly differ, since the right hand side of the equation bears no dependence on the (12) or (34) subscript. Thus, we find that, although in principle the group frequencies could differ, in practice the resources are distributed such that they are (at least to very good approximation) equal to one another. So then, now knowing that the two group frequencies must be equal to one another (i.e. $\Omega_{12} = \Omega_{34}$), it is clear that all $R'_i$ must also be equal, and therefore the only variance in natural frequency $\tilde{\omega} + \tilde{\sigma}\omega'_i + \tilde{\mu}R'_i$ will be due to the second term, and therefore the natural frequencies will be Gaussian distributed with variance equal to $\tilde{\sigma}^2$. This completes our discussion of the doubly-synchronized state.

## 3.2 Doubly-Unsynchronized

Next we consider the doubly-unsynchronized state, which is obtained as both $K_{12}$ and $K_{34}$ tend to 0. In this case the dynamics of the system are

$$\dot{\phi}_i = \tilde{\omega} + \tilde{\sigma}\omega'_i + \tilde{\mu}R'_i \tag{19}$$

$$\dot{R}'_i = B'_i - R'_i + \tilde{\beta}\dot{\phi}_i \tag{20}$$

$$\dot{B}'_i = p\sum_j C_{ij}(B'_j\dot{\phi}_i - B'_i\dot{\phi}_j). \tag{21}$$

Without the coupling term, this is a perfectly linear system of differential equations, which means analyzing it is relatively straightforward.

Recall the structure of $C$. We have either the high-high or high-low topology scenario. In both cases, all nodes within G1-G4 are internally connected, and then all nodes between either G1 and G3 (high-high) or G1 and G4 (high-low) are connected, and likewise for G2 and G4 (high-high) or G2 and G3 (high-low).

Thus, the $C$ matrix will be either

$$C = \begin{pmatrix} \mathbf{1} & \mathbf{0} & \mathbf{1} & \mathbf{0} \\ \mathbf{0} & \mathbf{1} & \mathbf{0} & \mathbf{1} \\ \mathbf{1} & \mathbf{0} & \mathbf{1} & \mathbf{0} \\ \mathbf{0} & \mathbf{1} & \mathbf{0} & \mathbf{1} \end{pmatrix} \quad \text{or} \quad C = \begin{pmatrix} \mathbf{1} & \mathbf{0} & \mathbf{0} & \mathbf{1} \\ \mathbf{0} & \mathbf{1} & \mathbf{1} & \mathbf{0} \\ \mathbf{0} & \mathbf{1} & \mathbf{1} & \mathbf{0} \\ \mathbf{1} & \mathbf{0} & \mathbf{0} & \mathbf{1} \end{pmatrix} , \tag{22}$$

where $\mathbf{0}$ and $\mathbf{1}$ are $N/4$-by-$N/4$ matrices of zeros and ones, respectively, and the ordering of the $C$ matrix is (G1,G2,G3,G4). In any case, due to the all-to-all nature of these blocks, it will be convenient to define averages of $\dot{\phi}$, $R'$, and $B'$ over each of the four groups. Call these $\langle\dot{\phi}\rangle_g$, $\langle R'\rangle_g$, and $\langle B'\rangle_g$, where $g = \{1, 2, 3, 4\}$ is the group label.

What is the advantage of this approach? Due to the block nature of the $C$ matrix, the bath dynamics will often only consider the averages of quantities rather than the independent values for each node. In particular, consider the bath dynamics of an oscillator in group $g$, and let $g'$ be the group connected to group $g$. We have

$$\dot{B}'_i = \frac{Np}{4}\Big( \big( \langle B'\rangle_g + \langle B'\rangle_{g'} \big)\dot{\phi}_i - \big( \langle\dot{\phi}_i\rangle_g + \langle\dot{\phi}_i\rangle_{g'} \big) B'_i \Big) . \tag{23}$$

Since we are dealing in averages, we can also take the average of both sides over group $g$, in which case we find

$$\langle\dot{B}'\rangle_g = \frac{Np}{4}\Big( \big( \langle B'\rangle_g + \langle B'\rangle_{g'} \big) \langle\dot{\phi}\rangle_g - \big( \langle\dot{\phi}_i\rangle_g + \langle\dot{\phi}_i\rangle_{g'} \big) \langle B'\rangle_g \Big) , \tag{24}$$

which can then be simplified to

$$\langle\dot{B}'\rangle_g = \frac{Np}{4}\Big( \langle B'\rangle_{g'} \langle\dot{\phi}\rangle_g - \langle\dot{\phi}_i\rangle_{g'} \langle B'\rangle_g \Big) . \tag{25}$$

Thus, in terms of the average bath levels, we have a biased diffusion process as well. Since biased diffusion has a unique equilibrium, we can see that, at equilibrium

$$\langle B'\rangle_g = \frac{2}{N} \frac{\langle\dot{\phi}\rangle_g}{\langle\dot{\phi}\rangle_g + \langle\dot{\phi}\rangle_{g'}} . \tag{26}$$

Now note that

$$\langle\dot{\phi}\rangle_g = \tilde{\omega} + \tilde{\sigma} \langle\omega'\rangle_g + \tilde{\mu} \langle R'\rangle_g , \tag{27}$$

and also that

$$\langle\dot{R}'\rangle_g = \langle B'\rangle_g - \langle R'\rangle_g + \tilde{\beta} \langle\dot{\phi}\rangle_g . \tag{28}$$

Between these two equations, it is clear that $\langle R'\rangle_g$ will undergo an exponential decay to the value $(1-\tilde{\beta}\tilde{\mu})^{-1}(\langle B'\rangle_g + \tilde{\beta}\tilde{\omega} + \tilde{\beta}\tilde{\sigma}\langle\omega'\rangle_g)$. Thus, once the system has equilibrated, we have

$$\langle\dot{\phi}\rangle_g = (1-\tilde{\beta}\tilde{\mu})^{-1}\Big( \tilde{\omega} + \tilde{\sigma} \langle\omega'\rangle_g + \tilde{\mu} \langle B'\rangle_g \Big) . \tag{29}$$

We may now combine Equations 26 and 29 to solve for $\langle B' \rangle_g$ and $\langle \dot{\phi} \rangle_g$. To do this, first consider $\langle \dot{\phi} \rangle_g + \langle \dot{\phi} \rangle_{g'}$. From Equation 29, we can write

$$\langle \dot{\phi} \rangle_g + \langle \dot{\phi} \rangle_{g'} = \left(1 - \tilde{\beta}\tilde{\mu}\right)^{-1} \left( 2\tilde{\omega} + \tilde{\sigma}(\langle \omega' \rangle_g + \langle \omega' \rangle_{g'}) + \tilde{\mu}\big( \langle B' \rangle_g + \langle B' \rangle_{g'} \big) \right). \tag{30}$$

Now, from Equation 26, it is clear that $\langle B' \rangle_g + \langle B' \rangle_{g'} = \frac{2}{N}$. The sum of $\langle \omega' \rangle$ terms will depend on whether we consider the high-high or high-low topology, so for now we will remain agnostic and leave it as is. Thus,

$$\langle \dot{\phi} \rangle_g + \langle \dot{\phi} \rangle_{g'} = \left(1 - \tilde{\beta}\tilde{\mu}\right)^{-1} \left( 2\tilde{\omega} + \tilde{\sigma}(\langle \omega' \rangle_g + \langle \omega' \rangle_{g'}) + \frac{2}{N}\tilde{\mu} \right). \tag{31}$$

Since this sum does not depend on $\langle \dot{\phi} \rangle$ or $\langle B' \rangle$, we can plug Equation 29 to simplify Equation 26 and solve for $\langle B' \rangle$. We find that

$$\langle B' \rangle_g = \frac{1}{N} \frac{\tilde{\omega} + \tilde{\sigma} \langle \omega' \rangle_g}{\tilde{\omega} + \frac{1}{2}\tilde{\sigma}(\langle \omega' \rangle_g + \langle \omega' \rangle_{g'})}. \tag{32}$$

In fact, we can generalize beyond the average. Equation 26 actually holds even if we consider an individual oscillator, rather than the average, so long as we replace $\langle \dot{\phi} \rangle_g$ in the numerator by $\dot{\phi}_i$. The denominator, however, is unchanged. As a consequence, Equation 32 also holds for an individual oscillator as long as we replace $\langle \omega' \rangle_g$ in the numerator by $\omega'_i$, but once again, the denominator stays the same. From this analysis, we now know the equilibrium bath level of oscillator $i$, which means we can determine the equilibrium resource level of oscillator $i$, and therefore the equilibrium frequency of oscillator $i$. Doing all of this, we come finally to the result presented in the main article:

$$\dot{\phi}_i = \left( \frac{\frac{\tilde{\mu}}{N} + \tilde{\omega} + \frac{1}{2}\tilde{\sigma}(\langle \omega' \rangle_g + \langle \omega' \rangle_{g'})}{(1 - \tilde{\beta}\tilde{\mu})(\tilde{\omega} + \frac{1}{2}\tilde{\sigma}(\langle \omega' \rangle_g + \langle \omega' \rangle_{g'})} \right)(\tilde{\omega} + \tilde{\sigma}\omega'_i). \tag{33}$$

Note, however, that the main article presented this result slightly differently to make the effect of bath topology more obvious. In particular, the $(\langle \omega' \rangle_g + \langle \omega' \rangle_{g'})/2$ term was rewritten as $\langle \omega' \rangle_{\pm/0}$. The motivation for this alteration is that $(\langle \omega' \rangle_g + \langle \omega' \rangle_{g'})/2$ is just the average of $\omega'$ among groups $g$ and $g'$. If we consider the high-high topology scenario, then $g$ and $g'$ will be either G1 and G3, or G2 and G4. Since G1 and G3 are on average faster and G2 and G4 on average slower, we can write the average as $\langle \omega' \rangle_{\pm}$, meaning the average of $\omega'$ over either the two fast groups (+) or the two slow groups (−). On the other hand, in the high-low topology scenario, the average will always be over one fast group and one slow group, hence the 0 subscript in that case. In fact, since $\omega'$ is Gaussian distributed with zero mean when considering a fast and slow group jointly, the average will be very nearly zero in the limit of many oscillators. This completes the discussion of the doubly-unsynchronized case.

## 3.3 Singly-Synchronized

Finally, we come to the most complex case considered in the article. In this case, we let one of $K_{12}$ or $K_{34}$ go to zero, while the other goes to infinity. Thus, one pair has no phase coupling, while the other pair is phase-locked. Further, we have, as usual, one of our two bath topologies creating an avenue of communication among the two pairs. Without loss of generality, suppose that the {G1,G2} pair is phase-locked, while the {G3,G4} pair have no phase interaction. Thus, all oscillators in {G1,G2} turn with some group velocity $\Omega$, while all oscillators in {G3,G4} turn at their natural frequencies.

Now, many of the equations from the previous section still hold in this case. In particular, we still have Equation 26

$$\langle B' \rangle_g = \frac{2}{N} \frac{\langle \dot{\phi} \rangle_g}{\langle \dot{\phi} \rangle_g + \langle \dot{\phi} \rangle_{g'}} \,. \tag{34}$$

However, Equation 27 no longer holds because we must now include the coupling term in that equation. It may seem strange to include that term since the coupling is supposed to be equal and opposite for Kuramoto oscillators. The reason it must be included is because G1 will generally have oscillators on the leading edge of the group getting pulled backwards, while G2 will generally have oscillators on the trailing side of the group getting pulled forwards. Thus, the average impact of the coupling term is not zero for the two groups independently, but generally negative for G1 and positive for G2, with the negative and positive contributions being of the same overall magnitude. For G3 and G4, however, Equation 27 holds as before.

So then how shall we modify Equation 27 for groups G1 and G2? Equation 27 just expresses the average frequency of the oscillators, and since G1 and G2 are synchronized, their average velocity is just the group frequency $\Omega$ for both groups. Further, $\Omega$ will just be the average natural frequency between G1 and G2. That is,

$$\Omega = \tilde{\omega} + \tilde{\mu} \frac{\langle R' \rangle_1 + \langle R' \rangle_2}{2} \,, \tag{35}$$

where we have neglected the $\tilde{\sigma}\omega'$ term because the average of that term among a fast group and a slow group jointly will be (very nearly) zero.

Further, for G1 and G2, the equilibrium internal resource levels will on average be

$$\langle R' \rangle_{1,2} = \langle B' \rangle_{1,2} + \tilde{\beta}\Omega \,. \tag{36}$$

Now plugging Equation 36 into Equation 35, we find

$$\Omega = (1 - \tilde{\beta}\tilde{\mu})^{-1} \left( \tilde{\omega} + \tilde{\mu} \frac{\langle B' \rangle_1 + \langle B' \rangle_2}{2} \right) . \tag{37}$$

We can use this to express Equation 34 as

$$\langle B' \rangle_{3,4} = \frac{2}{N} \frac{\langle \dot{\phi} \rangle_{3,4}}{\Omega + \langle \dot{\phi} \rangle_{3,4}} \,. \tag{38}$$

Further, $\langle\dot{\phi}\rangle_{3,4}$ is still given by Equation 29 from the last section. That is,

$$\langle\dot{\phi}\rangle_{3,4} = (1-\tilde{\beta}\tilde{\mu})^{-1}\left(\tilde{\omega} + \tilde{\sigma}\,\langle\omega'\rangle_{3,4} + \tilde{\mu}\,\langle B'\rangle_{3,4}\right). \tag{39}$$

Combining Equations 37–39, we find

$$\langle B'\rangle_{3,4} = \frac{2}{N}\frac{\tilde{\omega} + \tilde{\sigma}\,\langle\omega'\rangle_{3,4} + \tilde{\mu}\,\langle B'\rangle_{3,4}}{2\tilde{\omega} + \tilde{\sigma}\,\langle\omega'\rangle_{3,4} + \tilde{\mu}\,\langle B'\rangle_{3,4} + \tilde{\mu}\frac{\langle B'\rangle_1 + \langle B'\rangle_2}{2}}. \tag{40}$$

Here it will be convenient to abbreviate our notation somewhat. Let $\langle B'\rangle_+$ be the average bath level in G3 and $\langle B'\rangle_-$ be the average bath level in G4. Since G1 and G2 share a fixed supply of resources with G3 and G4, we know that $\langle B'\rangle_1 + \langle B'\rangle_2 = \frac{4}{N} - \langle B'\rangle_+ - \langle B'\rangle_-$. Then Equation 40 becomes

$$\langle B'\rangle_\pm = \frac{2}{N}\frac{\tilde{\omega} + \tilde{\sigma}\,\langle\omega'\rangle_\pm + \tilde{\mu}\,\langle B'\rangle_\pm}{2\tilde{\omega} + \tilde{\sigma}\,\langle\omega'\rangle_\pm + \frac{2\tilde{\mu}}{N} \pm \tilde{\mu}\frac{\langle B'\rangle_+ - \langle B'\rangle_-}{2}}. \tag{41}$$

If we now multiply the denominator onto both sides of the equation we have

$$(2\tilde{\omega}+\tilde{\sigma}\,\langle\omega'\rangle_\pm+\frac{2\tilde{\mu}}{N})\,\langle B'\rangle_\pm \pm\tilde{\mu}\frac{\langle B'\rangle_+ - \langle B'\rangle_-}{2}\,\langle B'\rangle_\pm = \frac{2}{N}(\tilde{\omega}+\tilde{\sigma}\,\langle\omega'\rangle_\pm+\tilde{\mu}\,\langle B'\rangle_\pm). \tag{42}$$

We can simplify this equation down to the following:

$$\langle B'\rangle_\pm^2 + \langle B'\rangle_\pm\left(\frac{4\tilde{\omega}}{\tilde{\mu}} + \frac{2\tilde{\sigma}\,\langle\omega'\rangle_\pm}{\tilde{\mu}} - \langle B'\rangle_\mp\right) - \frac{4}{N}\left(\frac{\tilde{\omega}}{\tilde{\mu}} + \frac{\tilde{\sigma}\,\langle\omega'\rangle_\pm}{\tilde{\mu}}\right) = 0. \tag{43}$$

This is Equation 18 from the main article, which we can solve numerically if need be.

In any case, now that we know $\langle B'\rangle_+$ and $\langle B'\rangle_-$ (at least in principle), we can find the frequencies of the unsynchronized oscillators and the natural frequencies of the synchronized oscillators. First, recall that $\langle B'\rangle_1 = \frac{2}{N} - \langle B'\rangle_{+/-}$, where the / indicates the high-high topology on the left and the high-low topology on the right. Likewise, $\langle B'\rangle_2 = \frac{2}{N} - \langle B'\rangle_{-/+}$. Since all the oscillators in G1 all travel at the same frequency $\Omega$, they will all have identical bath levels, and likewise all the oscillators in G2 will have identical bath levels. Thus, if we call the natural frequencies $\nu_{1i}$ and $\nu_{2i}$, we find

$$\nu_{1i} = \tilde{\omega} + \tilde{\sigma}\omega'_i + \tilde{\mu}\left(\frac{2}{N} - \langle B'\rangle_{+/-}\right), \tag{44}$$

and likewise

$$\nu_{2i} = \tilde{\omega} + \tilde{\sigma}\omega'_i + \tilde{\mu}\left(\frac{2}{N} - \langle B'\rangle_{-/+}\right). \tag{45}$$

From these, we see that the spreads are characterized by $\tilde{\sigma}$. However, the means are not equal, differing by the $\langle B'\rangle_{+/-}$ terms, and so the two groups G1 and

G2 will generally be shifted by different amounts, thus no longer forming a joint Gaussian distribution.

Next we consider the unsynchronized oscillator frequencies in G3 and G4. Call these $\dot{\phi}_{+i}$ (G3) and $\dot{\phi}_{-i}$ (G4). By arguments essentially equivalent to those in the doubly-unsynchronized section of this Supplement, we find that

$$\dot{\phi}_{\pm i} = \left(1 - \tilde{\beta}\tilde{\mu}\right)^{-1} \left[ \frac{\tilde{\mu} \left\langle B' \right\rangle_{\pm} + \tilde{\omega} + \tilde{\sigma} \left\langle \omega' \right\rangle_{\pm}}{\tilde{\omega} + \tilde{\sigma} \left\langle \omega' \right\rangle_{\pm}} \right] \left(\tilde{\omega} + \tilde{\sigma}\omega_i'\right), \tag{46}$$

which is the result presented in Equation 17 of the main article.

Now we turn to finding the approximate solution for the equilibrium bath levels $\langle B' \rangle_{\pm}$. In particular, we will assume that $\langle B' \rangle_{+}$ and $\langle B' \rangle_{-}$ are nearly equal, differing only by a symmetric displacement from some mean level. That is, we assume that

$$\left\langle B' \right\rangle_{\pm} = \alpha \pm \delta\,, \tag{47}$$

where $\delta \ll \alpha$.

Our strategy will simply be to plug this expression for $\langle B' \rangle_{\pm}$ into Equation 43, which is really two equations, and then to solve for the unknown $\alpha$ and $\delta$. Further, since $\delta \ll \alpha$, we will be able to neglect many terms to obtain a simpler expression than that in Equation 43. Performing the mentioned operations and neglecting any terms quadratic or greater in $\delta$, we obtain the following pair of equations:

$$\frac{4\tilde{\omega}}{\tilde{\mu}}\alpha + \frac{2\tilde{\sigma}\left\langle \omega' \right\rangle_{+}}{\tilde{\mu}}\delta - \frac{4}{N}\frac{\tilde{\omega}}{\tilde{\mu}} = 0 \tag{48}$$

$$2\alpha\delta + \frac{2\tilde{\sigma}\left\langle \omega' \right\rangle_{+}}{\tilde{\mu}}\alpha + \frac{4\tilde{\omega}}{\tilde{\mu}}\delta - \frac{4\tilde{\sigma}\left\langle \omega' \right\rangle}{N\tilde{\mu}} = 0\,. \tag{49}$$

Now from Equation 48 we can see that if $\tilde{\sigma}\langle \omega' \rangle_{+} \ll \tilde{\omega}$, then $\alpha = 1/N$, and the same condition in Equation 49 gives $\delta = 0$. From this, it is clear that the difference between $\langle B' \rangle_{+}$ and $\langle B' \rangle_{-}$ will be controlled by the size of $\tilde{\sigma}\langle \omega' \rangle_{+}$, which is quite sensible because this is the term which controls how different the fast and slow groups are from one another, with that difference being relative to the overall offset $\tilde{\omega}$. Thus, we will solve this pair of equations to linear order in $\tilde{\sigma}\langle \omega' \rangle$, which will suffice to give us the necessary intuition for the observed phenomena.

Upon doing so, we find

$$\left\langle B' \right\rangle_{\pm} \approx \frac{1}{N} \pm \frac{\tilde{\sigma}\left\langle \omega' \right\rangle}{\tilde{\mu} + \tilde{\omega}N}\,, \tag{50}$$

which is the result reported in the main article.
